# Supplementary material for: All-Optical Vector Atomic Magnetometer
Source: arXiv:1403.7545 source file (2014-03-28)
Supplement: Supplementary file 1 [file VectorMag_SM_sub.pdf]

# All-Optical Vector Atomic Magnetometer – Supplemental Material

B. Patton
*Department of Physics, University of California, Berkeley, CA 94720-7300 and Physik-Department, Technische Universität München, 85748 Garching, Germany*

E. Zhivun
*Department of Physics, University of California, Berkeley, CA 94720-7300*

D. C. Hovde
*Southwest Sciences Ohio Operations, Cincinnati, OH 45244*

D. Budker
*Department of Physics, University of California, Berkeley, CA 94720-7300 Nuclear Science Division, Lawrence Berkeley National Laboratory, Berkeley, CA 94720 and Helmholtz Institute, Johannes Gutenberg University, 55099 Mainz, Germany*
(Dated: March 28, 2014)

## I. EXPERIMENTAL DETAILS

Prior to each long-term measurement, the scalar sensitivity of the magnetometer was optimized through adjustment of the pump and probe beam powers and optical detunings. This optimum was found by measuring the signal-to-noise ratio of the magnetic-resonance curve and, independently, by stepping the local oscillator frequency by small amounts around $\omega_L$ and maximizing the resulting shift in the lock-in output. The optimal parameters for the pump and probe beams are relatively forgiving, and over a range of ∼1 GHz in optical frequency it is possible to achieve the same sensitivity by choosing appropriate beam powers. (Higher beam powers require greater detuning from the optical absorption line.)

For the measurements shown in Figs. 2 and 3, active feedback was used to control the $LS_y$ and $LS_z$ beam powers. Each light-shift beam has an optical pickoff outside the shields which directs a small fraction of the beam's power onto a photodiode. The resulting photocurrent is sent through a current preamplifier (Stanford Research Systems SR570) whose output voltage is measured by a PID controller (Stanford Research Systems SIM960) and compared to a set voltage given by an analog output of the data acquisition board. The output of the PID controller is sent to the AOM analog input, so that the observed optical power can be controlled by computer and modulated at frequencies in excess of 1 kHz. Prior to the experiment we measured the power of the $LS_y$ and $LS_z$ beams within the $\mu$-metal shields in order to convert these voltages into measured beam powers. For added precision, the measured beam powers are recorded during data acquisition. When processing the data, we take the Fourier transform of these recorded voltages in order to calculate each beam's power spectral density at its modulation frequency. The response of the lock-in output to each light-shift beam is normalized according to this measurement.

## II. LIGHT SHIFTS

As thoroughly described in the literature [S1–S3], the AC Stark shift $\delta E$ of a ground-state alkali atom can be decomposed as:

$$\delta E = (\delta E)_0 + \delta\mathcal{A}\,\mathbf{I}\cdot\mathbf{S} + \boldsymbol{\mu}\cdot\mathbf{B}_{\rm LS} + (\delta E)_t, \qquad \text{(S1)}$$

where the first two terms represent, respectively, the scalar shift of all ground-state sublevels and the modification of the ground-state hyperfine coupling coefficient $\mathcal{A}$ between the nuclear and electron spins $\mathbf{I}$ and $\mathbf{S}$. As these terms do not affect Zeeman coherences within a single hyperfine manifold, we shall ignore them in the present discussion. The third term in Eq. (S1) represents the vector light shift, often described as a fictitious magnetic field $\mathbf{B}_{\rm LS}$ oriented along the propagation direction of a circularly polarized laser beam and coupling with the atomic spin $\boldsymbol{\mu}$. The tensor light shift $(\delta E)_t$ is caused by the quasiuniform electric field of the light producing second-order Stark shifts in the alkali sublevels, producing energy-level corrections akin to an added nonlinear Zeeman shift [S4].

Here we briefly remind the reader of the effect of a circularly polarized near-resonant beam incident upon an alkali vapor. Although it is sometimes claimed that only the vector light shift acts upon the alkali sublevels in this case, the effects of such a beam are distinct from those of an applied static magnetic field. We illustrate this with an atomic system with total angular momentum $F = 1$ in the lower state and $F' = 0$ in the upper state (Fig. S1). The left diagram in Fig. S1 shows the Zeeman effect of the $F = 1$ sublevels in a magnetic field applied along the quantization axis. The energy-level shift is proportional to the magnetic quantum number $m_F$. The right diagram in Fig. S1 shows the effect of a $\sigma_+$ circularly polarized beam red-detuned from the optical resonance. According to the selection rules for optical transitions, only the $m_F = -1$ sublevel is shifted in the lower-state manifold, resulting in a different splitting pattern from that

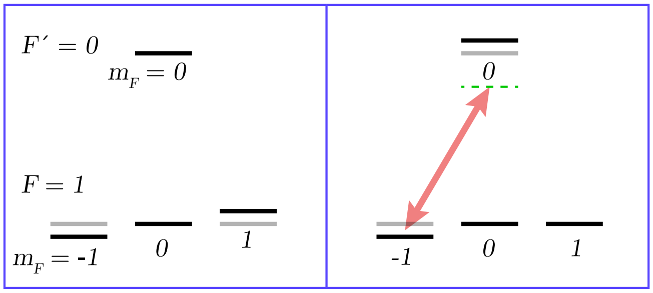


FIG. S1. Comparison between the Zeeman shift induced by a static magnetic field along the axis of quantization (left) and the AC Stark shift induced on the same system by a circularly polarized beam propagating along the same axis (right). The beam is red-detuned from the $F = 1 \rightarrow F' = 0$ transition. Energy levels are not to scale. Light grey bars represent unperturbed energy levels.

caused by the Zeeman effect. The overall light shift can be described as a combination of the vector and tensor terms in Eq. (S1), even for the present case of circularly polarized light. More generally, one can understand the difference in the Zeeman and the AC Stark effect from the perspective of an irreducible tensor basis. A detailed discussion may be found in Ref. [S5].

Many prior studies of the vector light shift have downplayed the tensor contribution to the AC Stark shift [S1, S2, S6], an approximation which can be justified when the excited-state hyperfine structure of the alkali atom (total angular momentum $F > 1/2$) is unresolved [S7]. Other studies [S8, S9] have restricted treatment of the AC Stark shift to highly symmetric conditions (e.g., wherein the pump beam, mean alkali spin projection, and magnetic field are all nearly collinear). Furthermore, nearly all discussions of the light shift ignore the light shift due to real transitions [S10], a justifiable assumption when the optical pumping rate of the light-shift beam is vanishingly small. Our experiment is a distinct violation of many of the above simplifying assumptions, since our magnetometer is based upon synchronous transverse pumping of alkali atoms within an evacuated vapor cell and a near-resonant transverse light-shift beam. Nevertheless, the good agreement between the data shown in Fig. 2 and the curve predicted by Eq. (3) validates the interpretation of the vector light shift as a fictitious magnetic field in the present context. We observed no measurable splitting of the magnetic resonance due to the $LS_y$ and $LS_z$ beams, so any corrections due to the tensor light shift are small enough to be neglected here. We also estimate the light shift due to real transitions to be extremely small, since the observed broadening of the magnetic-resonance line by the light-shift beams $LS_y$ and $LS_z$ is less than 1 Hz. The light shift due to real transitions is proportional to this decoherence rate, but smaller by a factor of $|\omega_e - \omega_g|/\Gamma$, where $\omega_g$ and $\omega_e$ are the ground-state and excited-state spin-precession frequencies and $\Gamma$ is the natural linewidth of the optical transition [S11, S12]. Because this factor is $\lesssim 10^{-3}$ for the magnetic fields used in this experiment, we can ignore this effect in the present experiment.

Future measurements are planned to quantify the small corrections to the magnetometer response caused by the tensor light shift, the light shift due to real transitions, and the quadratic correction $\zeta$ given in Eq. (2).

## III. UNCERTAINTY IN MEASUREMENT OF $\theta$

In the course of our measurement, we observe the shift in observed magnetic field due to the $LS_y$ light-shift beam and that due to the $LS_z$ light-shift beam. Denote these two shifts as $\Delta_y$ and $\Delta_z$, respectively. Once again taking only the lowest-order terms in the expansion of Eq. (1), we have:

$$f = \frac{\Delta_y}{\Delta_z} = \frac{1}{\beta}\tan\theta, \tag{S2}$$

where $\beta \equiv P_z\alpha_z/P_y\alpha_y$ is the ratio of effective fields of the $LS_z$ and $LS_y$ beams, ostensibly a constant on the order of unity. The precision of our measurement of $\Delta_y$ and $\Delta_z$ is the same as the precision of our scalar magnetometer, which we define as $\delta B_0$. This scalar sensitivity has no dependence on the primary field magnitude $B_0$, since the synchronous transverse pumping scheme operates equivalently over a wide range of magnetic fields [S13]. In the present analysis we also ignore any directional dependence of $\delta B_0$, which in general arises from the orientation of the pump and probe beams (not the $LS_y$ and $LS_z$ beams) with respect to the ambient field. For the sake of argument, one could reorient the pump and probe beams to optimize the scalar sensitivity of the magnetometer, or use a more advanced method of eliminating so-called "dead zones" in the magnetometer's sensitivity [S14].

Here we wish to calculate the uncertainty in the measurement of the magnetic-field angle $\theta$. Since $\theta = \arctan(\beta f)$, the uncertainty in $\theta$, denoted $\sigma_\theta$, is given by:

$$\sigma_\theta = \beta\sigma_f \frac{1}{1+\beta^2 f^2}, \tag{S3}$$

where $\sigma_f$ is the corresponding uncertainty in the measurement of $f$:

$$\begin{aligned}\sigma_f &= f\left[\frac{(\delta B_0)^2}{\Delta_y^2} + \frac{(\delta B_0)^2}{\Delta_z^2}\right]^{1/2} \\ &= \frac{\delta B_0}{\Delta_z^2}\sqrt{\Delta_y^2+\Delta_z^2}.\end{aligned} \tag{S4}$$

Combining this with Eq. (S3), we arrive at the expression for the uncertainty in the field angle:

$$\sigma_\theta = \delta B_0 \frac{\beta}{\Delta_z^2+\beta^2\Delta_y^2}\sqrt{\Delta_y^2+\Delta_z^2}. \tag{S5}$$

For the nominal case of $\beta = 1$, Eq. (S5) reduces to a particularly simple form:

$$\sigma_\theta = \delta B_0 \sqrt{\frac{1}{\Delta_y^2 + \Delta_z^2}} = \frac{\delta B_0}{B_{\mathrm{LS}}}, \tag{S6}$$

where $B_{\mathrm{LS}}$ is the magnitude of the magnetic field produced by each light-shift beam. In this case the uncertainty in the field angle depends neither on the magnitude $B_0$ of the ambient field nor on its angle $\theta$ with respect to the light-shift beams. Even if $\beta \neq 1$, this only introduces a directional dependence in the uncertainty $\sigma_\theta$, which still remains independent of the field magnitude. This remains true for a three-dimensional vector measurement, and can be understood intuitively as a consequence of the fact that some linear combination of the light-shift fields will always add in parallel with the primary field.

For the experimental technique used to measure the data shown in Figs. 2 and 3, the light-shift beams must shift the magnetic resonance only by a small amount, such that the lock-in Y output remains linearly proportional to the shift in Larmor frequency. This places a constraint on $B_{\mathrm{LS}}$, which must be smaller than the magnetic-resonance linewidth (in field units). Assuming that the light-shift beams had a maximum effective field of 0.286 nT (equivalent to a 1 Hz shift in spin-precession frequency), a magnetometer with scalar sensitivity of 50 fT/$\sqrt{\mathrm{Hz}}$ would have an angular precision of $\sim$175 $\mu$rad/$\sqrt{\mathrm{Hz}}$ .


[S1] B. S. Mathur, H. Tang, and W. Happer, Phys. Rev. **171**, 11 (1968).

[S2] C. Cohen-Tannoudji and J. Dupont-Roc, Phys. Rev. A **5**, 968 (1972).

[S3] W. Happer, Progress in Quantum Electronics **1**, 51 (1970).

[S4] K. Jensen, V. M. Acosta, J. M. Higbie, M. P. Ledbetter, S. M. Rochester, and D. Budker, Phys. Rev. A **79**, 023406 (2009).

[S5] M. Auzinsh, D. Budker, and S. Rochester, in *Optically Polarized Atoms — Understanding Light-Atom Interactions* (Oxford University Press, New York, NY, 2010), Chap. 19, iSBN 978-0-19-956512-2.

[S6] C. Y. Park, H. Noh, C. M. Lee, and D. Cho, Phys. Rev. A **63**, 032512 (2001).

[S7] Experimentally, this is generally the case when buffer gases are included in the alkali-vapor cell, or when a broad-spectrum discharge lamp acts as the source of the light-shift beam.

[S8] W. Happer and S. Svanberg, Phys. Rev. A **9**, 508 (1974).

[S9] J. Skalla, S. Lang, and G. Wackerle, Journal Of The Optical Society Of America B-Optical Physics **12**, 772 (1995).

[S10] B. R. Bulos, A. Marshall, and W. Happer, Phys. Rev. A **4**, 51 (1971).

[S11] C. Cohen-Tannoudji, Annales de Physique **7**, 423 (1962).

[S12] C. Cohen-Tannoudji, Annales de Physique **7**, 469 (1962).

[S13] This approximation begins to break down at geophysical fields (e. g. , 100 $\mu$T and above), where the nonlinear Zeeman splitting begins to change the structure of the magnetic resonance.

[S14] A. Ben-Kish and M. V. Romalis, Phys. Rev. Lett. **105**, 193601 (2010).
